# Supplementary material for: The Effective Fragment Molecular Orbital Method for Fragments Connected by Covalent Bonds
Source: arXiv:1202.4935 source file (2012-06-02)
Supplement: Supplementary file 1 [file supplimentary.pdf]

# Supplimentary Information: The Effective Fragment Molecular Orbital Method for Fragments Connected by Covalent Bonds

Casper Steinmann[1,*], Dmitri G. Fedorov[2], Jan H. Jensen[3]

**1 Department of Chemistry, University of Copenhagen, Universitetsparken 5, 2100 Copenhagen, Denmark**

**2 NRI, National Institute of Advanced Industrial Science and Technology (AIST), 1-1-1 Umezono, Tsukuba, Ibaraki 305-8568, Japan**

**3 Department of Chemistry, University of Copenhagen, Universitetsparken 5, 2100 Copenhagen, Denmark**

∗ **E-mail: steinmann@chem.ku.dk**

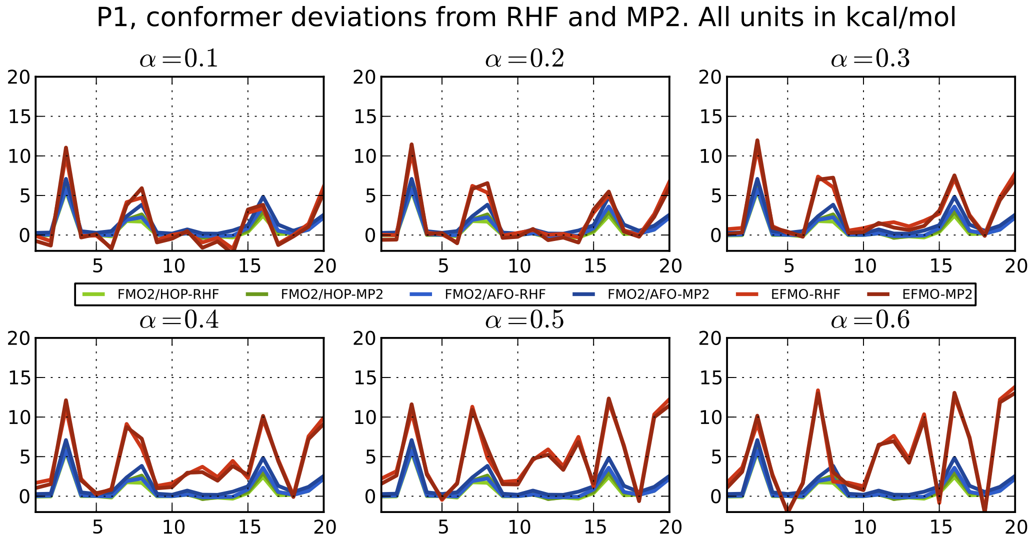


**Figure S1.** Deviations in energy from RHF and MP2 calculations of FMO2/HOP, FMO2/AFO and EFMO for the peptide P1 using two residues per fragment for different values of the screening parameter $\alpha$.

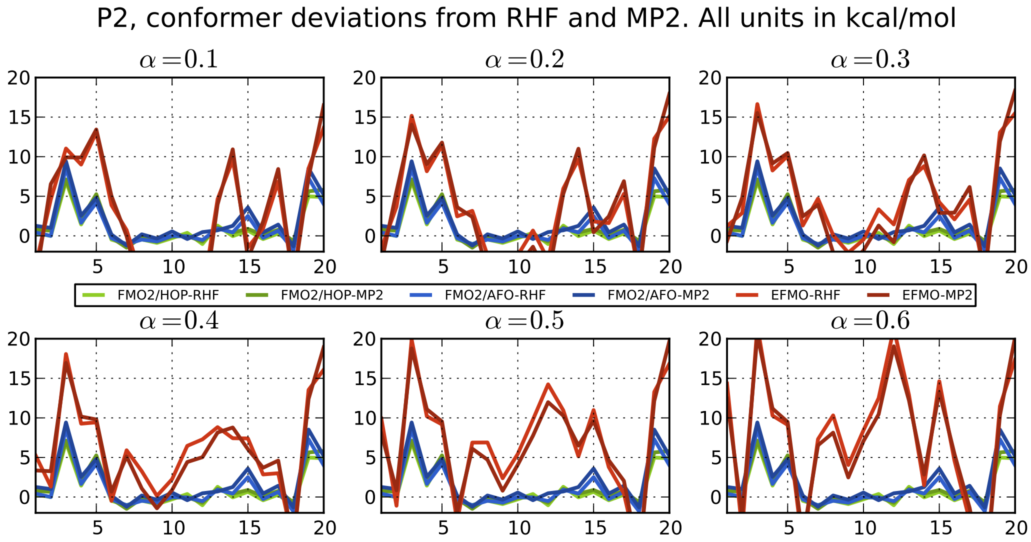


**Figure S2.** Deviations in energy from RHF and MP2 calculations of FMO2/HOP, FMO2/AFO and EFMO for the peptide P2 using two residues per fragment for different values of the screening parameter $\alpha$. Large positive values (>> 200 kcal/mol) indicates that EFMO did not converge. See main text for full details.

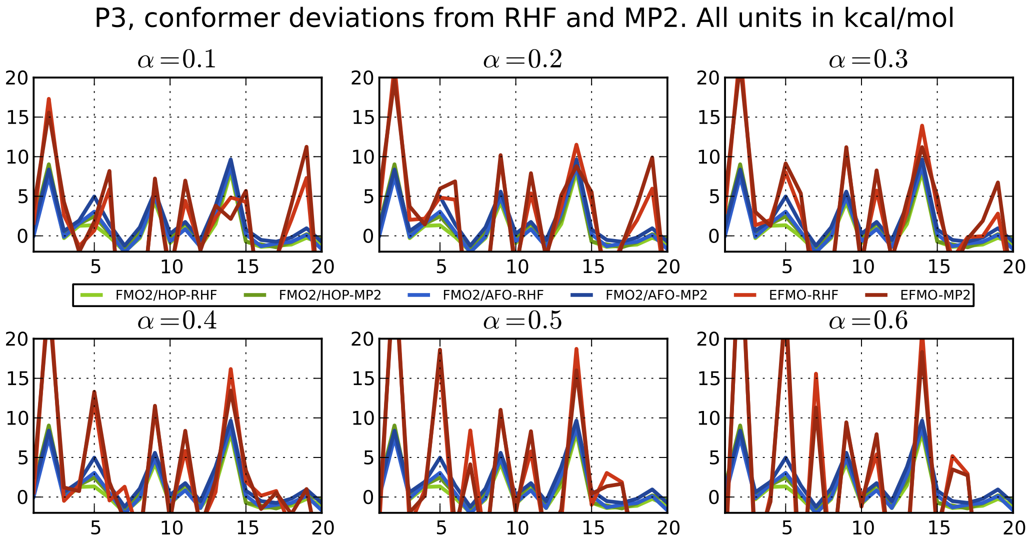


**Figure S3.** Deviations in energy from RHF and MP2 calculations of FMO2/HOP, FMO2/AFO and EFMO for the peptide P3 using two residues per fragment for different values of the screening parameter $\alpha$. Large positive values (>> 200 kcal/mol) indicates that EFMO did not converge. See main text for full details.

To measure how curled up a protein is, we use the radius of gyration $R_g^2$ given as

$$R_g^2 = \frac{1}{N_A}\sum_{k=1}^{N_A}(\vec{r}_k - \vec{r}_{\text{mean}})^2 \tag{S1}$$

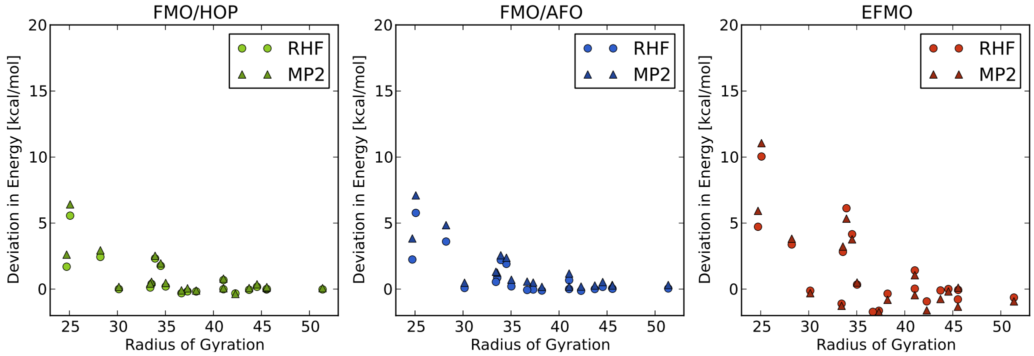


**Figure S4.** Correlation between the deviation in energy of peptide P1 using two residues per fragment and the radius of gyration. Lower values of the radius of gyration is a more compact protein.

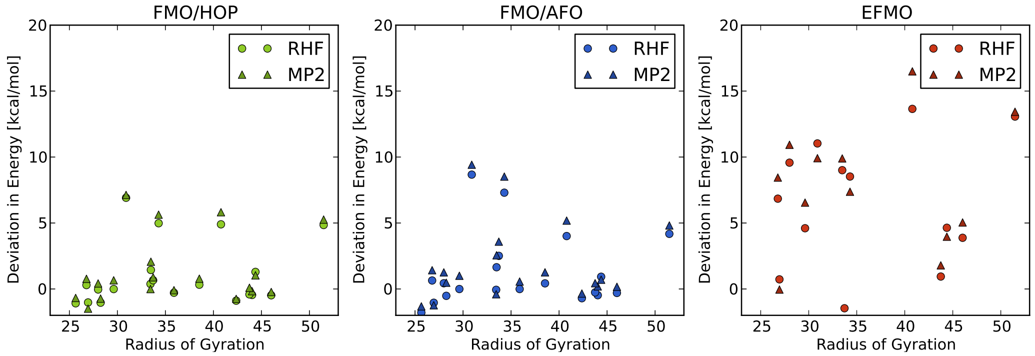


**Figure S5.** Correlation between the deviation in energy of peptide P2 using two residues per fragment and the radius of gyration. Lower values of the radius of gyration is a more compact protein.

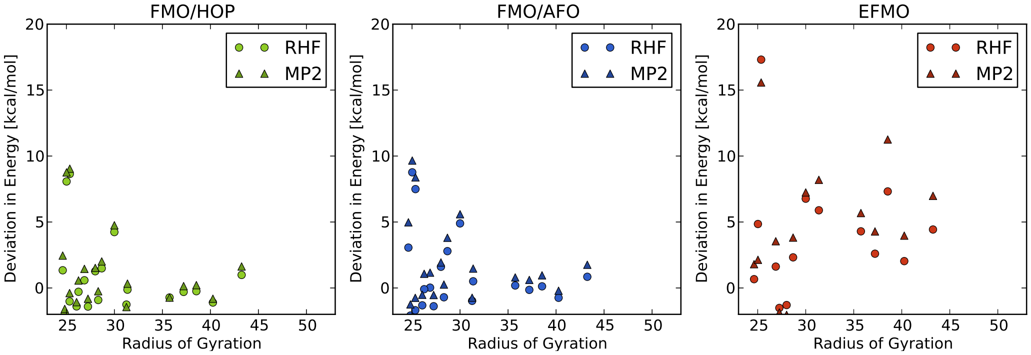


**Figure S6.** Correlation between the deviation in energy of peptide P3 using two residues per fragment and the radius of gyration. Lower values of the radius of gyration is a more compact protein.

**Table S1.** Calculated mean average deviation $\Delta E_{\mathrm{MAD}}$ and average deviation $\Delta E_{\mathrm{avg}}$ for conformers of the peptides P1, P2 and P3 using two residues per fragment, the 6-31G(d) basis set and different values of the screening parameter $\alpha$. For reference, FMO2/HOP and FMO2/AFO was included. All units in kcal/mol

| | P1 | | P2 | | P3 | |
|---|---|---|---|---|---|---|
| $\Delta E_{\mathrm{MAD}}$ | RHF | MP2 | RHF | MP2 | RHF | MP2 |
| FMO2/HOP | 0.82 | 1.01 | 1.59 | 1.73 | 1.87 | 2.00 |
| FMO2/AFO | 0.94 | 1.45 | 1.80 | 2.24 | 1.97 | 2.32 |
| EFMO($\alpha = 0.1$) | 2.02 | 2.33 | 6.28 | 7.28 | 5.94 | 7.10 |
| EFMO($\alpha = 0.2$) | 2.13 | 2.36 | 5.76 | 6.56 | 5.95 | 7.03 |
| EFMO($\alpha = 0.3$) | 2.99 | 2.88 | 5.65 | 6.03 | 5.35 | 6.43 |
| EFMO($\alpha = 0.4$) | 4.20 | 4.08 | 6.71 | 6.54 | 5.30 | 5.64 |
| EFMO($\alpha = 0.5$) | 5.27 | 5.14 | 8.41 | 7.92 | 8.04 | 7.08 |
| EFMO($\alpha = 0.6$) | 5.86 | 5.69 | 10.32 | 9.58 | 11.81 | 10.87 |
| $\Delta E_{\mathrm{avg}}$ | RHF | MP2 | RHF | MP2 | RHF | MP2 |
| FMO2/HOP | 0.71 | 0.96 | 1.02 | 1.32 | 0.79 | 1.29 |
| FMO2/AFO | 0.90 | 1.45 | 1.28 | 1.91 | 1.06 | 1.92 |
| EFMO($\alpha = 0.1$) | 1.28 | 1.15 | 2.37 | 2.10 | 0.07 | 0.35 |
| EFMO($\alpha = 0.2$) | 2.00 | 1.87 | 3.88 | 3.61 | 2.14 | 2.42 |
| EFMO($\alpha = 0.3$) | 2.98 | 2.85 | 4.88 | 4.61 | 2.72 | 3.00 |
| EFMO($\alpha = 0.4$) | 4.20 | 4.07 | 6.07 | 5.80 | 2.56 | 2.84 |
| EFMO($\alpha = 0.5$) | 5.18 | 5.05 | 7.21 | 6.94 | 1.68 | 1.95 |
| EFMO($\alpha = 0.6$) | 5.37 | 5.24 | 7.86 | 7.58 | -0.08 | 0.20 |

**Table S2.** Energy Error of EFMO and FMO2/AFO compared to *ab initio* calculations on proteins and protein-like structures for different values of $R_{\text{resdim}} = R_{\text{cor}}$ using one residue per fragment. In all calculations, the screening parameter $\alpha$ was kept fixed at a value of $\alpha = 0.1$

| | EFMO | | | | | | FMO2/AFO | |
|---|---|---|---|---|---|---|---|---|
| | $R_{\text{resdim}} = 1.0$ | | $R_{\text{resdim}} = 1.5$ | | $R_{\text{resdim}} = 2.0$ | | $R_{\text{resdim}} = 2.0$ | |
| | RHF | MP2 | RHF | MP2 | RHF | MP2 | RHF | MP2 |
| $\alpha$-(ALA)$_{10}$ | -9.82 | -4.65 | -9.59 | -5.44 | -9.59 | -5.44 | 0.44 | 6.52 |
| $\beta$-(ALA)$_{10}$ | 11.60 | 19.66 | 12.59 | 16.11 | 12.59 | 16.11 | -0.03 | 2.69 |
| $\alpha$-(ALA)$_{20}$ | -20.71 | -16.49 | -20.17 | -14.30 | -20.17 | -14.30 | -0.18 | 13.49 |
| $\beta$-(ALA)$_{20}$ | 26.58 | 44.85 | 28.78 | 36.81 | 28.78 | 36.81 | 0.05 | 6.40 |
| $\alpha$-(ALA)$_{40}$ | -40.60 | -39.91 | -39.46 | -31.79 | -39.46 | -31.79 | -1.53 | 26.99 |
| $\beta$-(ALA)$_{40}$ | 56.53 | 95.24 | 61.15 | 78.22 | 61.15 | 78.22 | 0.15 | 13.77 |
| Chignolin | 8.06 | 28.93 | 5.71 | 14.04 | 5.68 | 12.92 | 2.26 | 8.04 |
| Trp-cage | -9.58 | 44.36 | 4.11 | 17.34 | 3.90 | 16.38 | 10.34 | 26.58 |
| Crambine[a] | 4.00 | 124.98 | 12.86 | 42.81 | 12.85 | 40.60 | 12.78 | 53.90 |

[a]based on an FMO3-MP2/6-31G(d) calculation.

**Table S3.** Energy Error of EFMO compared to *ab initio* calculations on proteins and protein-like structures for different values of $R_{\text{resdim}} = R_{\text{cor}}$ using two residue per fragment. In all calculations, the screening parameter $\alpha$ was kept fixed at a value of $\alpha = 0.1$

| | EFMO | | | | | | FMO2/AFO | |
|---|---|---|---|---|---|---|---|---|
| | $R_{\text{resdim}} = 1.0$ | | $R_{\text{resdim}} = 1.5$ | | $R_{\text{resdim}} = 2.0$ | | $R_{\text{resdim}} = 2.0$ | |
| | RHF | MP2 | RHF | MP2 | RHF | MP2 | RHF | MP2 |
| $\alpha$-(ALA)$_{10}$ | -2.94 | 0.32 | -2.94 | -0.32 | -2.94 | 0.32 | -0.77 | -0.08 |
| $\beta$-(ALA)$_{10}$ | 0.60 | 0.89 | 0.60 | 0.89 | 0.60 | 0.89 | 0.08 | 0.25 |
| $\alpha$-(ALA)$_{20}$ | -2.75 | -9.66 | -2.75 | -9.66 | -2.75 | -9.66 | -2.30 | -0.53 |
| $\beta$-(ALA)$_{20}$ | 1.74 | 2.78 | 1.74 | 2.78 | 1.74 | 2.78 | 0.22 | 0.71 |
| $\alpha$-(ALA)$_{40}$ | 0.18 | -18.94 | 0.18 | -18.94 | 0.18 | -18.94 | -5.47 | -1.62 |
| $\beta$-(ALA)$_{40}$ | 4.05 | 6.46 | 4.05 | 6.46 | 4.05 | 6.46 | 0.51 | 1.62 |
| Chignolin | 1.57 | 4.84 | 1.79 | 1.48 | 1.79 | 1.48 | 0.37 | 1.38 |
| Trp-cage | -7.82 | 7.73 | -2.68 | -4.23 | -2.83 | -4.27 | 1.74 | 6.35 |
| Crambine[a] | 8.44 | 56.02 | 15.63 | 27.89 | 15.66 | 26.23 | 3.45 | 25.59 |

[a]based on an FMO3-MP2/6-31G(d) calculation.

# 1 Percentage Based Distribution of Induced Dipole Gradients

To improve the quality of the EFMO gradient, specifically from induced dipoles which are located in LMO-centroids, we implemented a percentage based distribution of the gradient between the two nearest atoms to the induced dipole instead of the current (transfer all to the nearest only). This is only in effect if the induced dipole is situated between two atoms, and not only near one (such as the case for a lone-pair on Oxygen for example).

Figure S7 shows the details. Here, $\vec{R}$ is the vector connecting the two atoms of interest, $\vec{R}_{\mu^{ind}}$ shows the location of the induced dipole $\vec{\mu}_{ind}$. Note that it is not nescessarily situated on the bond midpoint. The distribution of the gradient is based on a projection of the vectors from either atom to the induced dipole ($\vec{R}_1$ or $\vec{R}_2$) onto the vector $\vec{R}$, obtaining new vectors $\vec{R}_{1p}$ or $\vec{R}_{2p}$

From this, a single percentage of bondlength is obtained and the "amount" of gradient on atom $C_1$ is

$$\frac{\partial E^{ind}}{\partial \mathrm{C}_1} = \left(1 - \frac{|\vec{R}_{1p}|}{|\vec{R}|}\right) \frac{\partial E^{ind}}{\partial \vec{R}_{LMO}} \tag{S2}$$

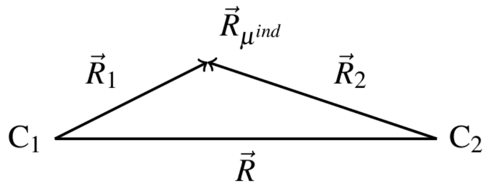


**Figure S7.** Two Carbon atoms ($C_1$ and $C_2$) and an the location of an induced dipole $\mu^{ind}$ above the bond midpoint (Drawn cartoonishly to emphasize the methodology).

# References


1. Steinmann C, Fedorov D, Jensen J (2010) Effective fragment molecular orbital method: A merger of the effective fragment potential and fragment molecular orbital methods. The Journal of Physical Chemistry A .
